# Supplementary material for: You can monitor your hydration level using your smartphone camera
Source: arXiv:2402.07467 source file (2024-02-12)
Supplement: Supplementary file 1 [file appendix.tex]

\section{}
